# Supplementary material for: Dynamic Byzantine-Robust Learning: Adapting to Switching Byzantine Workers
Source: arXiv:2402.02951 source file (2024-06-16)
Supplement: Supplementary file 1 [file adaptive_mfm_aggr.tex]

\section{Analysis of \Cref{alg:method-new} with MFM and AdaGrad}
Following the methodology outlined in \Cref{app:general}, this section focuses on analyzing \Cref{alg:method-new} under \textbf{Option 2}. Here, we replace the general $(\delta, \kappa)$-robust aggregator with the MFM aggregator and incorporate the adaptive AdaGrad learning rate~\cite{levy2017online,ward2020adagrad,attia2023sgd}. 

Recall that \Cref{alg:method-new} with \textbf{Option 2} and with AdaGrad learning rate as defined in \Cref{eq:adagrad} performs the following update rule for every $t\in\sbrac{T}$:
\begin{align}
    & J_t\sim\text{Geom}(\nicefrac{1}{2}) \nonumber \\
    & \widehat{g}_t^{j}\gets \text{MFM}(\widebar{g}_{t,1}^{j},\ldots,\widebar{g}_{t,m}^{j}; \T^{j}), \quad \T^j = 4\V\sqrt{\frac{2\log\brac{16m^2 T}}{2^j}} \label{eq:mfm_aggregated_grad} \\
    & g_t \gets  \widehat{g}_t^{0} + \begin{cases}
        2^J_t\brac{\widehat{g}_t^{J_t} - \widehat{g}_t^{J_t-1}}, &\text{if } J_t\leq\Jmax\coloneqq\floor{\log{T}} \text{ and } \Ecal_t(J_t) \text{ holds} \\
        0, &\text{otherwise}
    \end{cases} \label{eq:mlmc_agg_mfm} \\
    & x_{t+1} \gets \proj{\K}{x_t - \eta_t g_t }, \quad \eta_t = \frac{\eta_0}{\sqrt{\sum_{s=1}^{t}{\norm{g_s}^2}}}\; ,  \label{eq:adagrad_update}
\end{align}
where the associated event $\Ecal_t(J_t)$ in this case is defined as,
\begin{equation}\label{eq:event_E_option2}
    \Ecal_t(J_t)\coloneqq \cbrac{\lVert \widehat{g}_t^{J_t} - \widehat{g}_t^{J_t-1}\rVert\leq \frac{3\tilde{C}\V}{\sqrt{2^{J_t}}}}, \quad \tilde{C}= 32\sqrt{\log{\brac{32m^2 T}}}\; .
\end{equation}

Similarly to \Cref{app:general}, prior to presenting the convergence results, we establish first and second orders properties of the MLMC estimator, mirroring \Cref{lem:mlmc_1st_general,lem:2nd_order_aggr,lem:mlmc_2nd_general}.

\begin{lemma}[MLMC Bias -- MFM Aggregator]\label{lem:mlmc_1st_mfm}
    Consider the MLMC gradient estimator in \Cref{eq:mlmc_agg_mfm}. For every $t\notin\badrounds$, it holds that
    \[
        \E_{t-1}[g_t] = \E_{t-1}[\widehat{g}_t^{\Jmax}] - y_t\; ,
    \]
    where $y_t$ satisfies: 
    \[
        \norm{y_t} \leq \frac{(\tilde{C}\V + \norm{\nabla_t})\log{T}}{mT} \; .
    \]
\end{lemma}
\begin{proof}
    By replicating the steps outlined in the proof of \Cref{lem:mlmc_1st_general}, we obtain $\E_{t-1}[g_t] = \E_{t-1}[\widehat{g}_t^{\Jmax}] - y_t$, where $y_t=\sum_{j=1}^{\Jmax}{z_t^{j}}$ and $z_t^{j} = \E_{t-1}[\widehat{g}_t^{j} - \widehat{g}_t^{j-1} | \Ecal_t(j)^c]\prob_{t-1}(\Ecal_t(j)^{c})$. 
    While the event $\Ecal_t$ is slightly different, we follow similar steps, replacing \Cref{lem:core_lemma} with \Cref{lem:mfm}. By item 1 of \Cref{lem:mfm}, for every $j=0,\ldots,\Jmax$ we have that $\lVert{\widehat{g}_t^{j} - \nabla_t}\rVert\leq \sqrt{100\log\brac{16m^2 T}\V^2 + \norm{\nabla_t}^2} \leq 10\sqrt{\log\brac{16m^2 T}}\V + \norm{\nabla_t}$, implying that $\lVert{\widehat{g}_t^{j} - \widehat{g}_t^{j-1}}\rVert \leq 20\sqrt{\log\brac{16m^2 T}}\V + 2\norm{\nabla_t}$. In addition, item 2 of \Cref{lem:mfm} implies that 
    \[
        \prob_{t-1}\brac{\lVert{\widehat{g}_t^{j} - \nabla_t}\rVert\leq \tilde{C}\V\sqrt{\frac{\tilde{\gamma}}{2^{j}}}} \geq 1 - \frac{1}{4mT}, \quad \forall j=0,\ldots,\Jmax, \quad\text{ where } \tilde{\gamma} = \frac{1}{m} + \delta^2\; .
    \]
    Applying the union bound enables to bound $\prob_{t-1}(\Ecal_t(j)^c)$ as follows:
    \begin{align*}
        \prob_{t-1}\brac{\Ecal_t(j)^c} &= \prob_{t-1}\brac{\lVert \widehat{g}_t^{j} - \widehat{g}_t^{j-1} \rVert > \frac{3\tilde{C}\V}{\sqrt{2^{j}}}} \\ &\leq \prob_{t-1}\brac{\lVert \widehat{g}_t^{j} - \widehat{g}_t^{j-1} \rVert > (1+\sqrt{2})\tilde{C}\V\sqrt{\frac{\tilde{\gamma}}{2^{j}}}} \\ &\leq \prob_{t-1}\brac{\cbrac{\lVert \widehat{g}_t^{j} - \nabla_t\rVert> \tilde{C}\V\sqrt{\frac{\tilde{\gamma}}{2^{j}}}}\bigcup \cbrac{\lVert \widehat{g}_t^{j-1} - \nabla_t \rVert> \tilde{C}\V\sqrt{\frac{\tilde{\gamma}}{2^{j-1}}}}} \\ &\leq \prob_{t-1}\brac{\lVert \widehat{g}_t^{j} - \nabla_t\rVert> \tilde{C}\V\sqrt{\frac{\tilde{\gamma}}{2^{j}}}} + \prob_{t-1}\brac{\lVert \widehat{g}_t^{j-1} - \nabla_t\rVert> \tilde{C}\V\sqrt{\frac{\tilde{\gamma}}{2^{j-1}}}} \\ &\leq \frac{1}{4mT} + \frac{1}{4mT} = \frac{1}{2mT}\; .
    \end{align*}
    where the second inequality follows from $(1 + \sqrt{2})\sqrt{\tilde{\gamma}}\leq (1 + \sqrt{2})\sqrt{\nicefrac{5}{4}}\leq 3$ as $\tilde{\gamma}=\delta^2 + \nicefrac{1}{m} \geq \nicefrac{5}{4}$. Combining the bounds on $\lVert \widehat{g}_t^{j} - \widehat{g}_t^{j-1}\rVert$ and $\prob_{t-1}(\Ecal_t(j)^c)$ gives:
    \begin{align*}
        \lVert{z_t^j}\rVert \leq\!\E_{t-1}[\lVert \widehat{g}_t^{j} - \widehat{g}_t^{j-1}\rVert | \Ecal_t(j)^c]\prob_{t-1}(\Ecal_t(j)^c)\leq\frac{20\sqrt{\log\brac{16m^2 T}}\V + 2\norm{\nabla_t}}{2mT} = \frac{10\V\sqrt{\log\brac{16m^2T}}}{mT} + \frac{\norm{\nabla_t}}{mT}\; .
    \end{align*}
    This implies, by the triangle inequality, that
    \begin{align*}
        \norm{y_t}\leq\sum_{j=1}^{\Jmax}{\lVert z_t^{j} \rVert} \leq \brac{\frac{10\V\sqrt{\log\brac{16m^2 T}}}{mT} + \frac{\norm{\nabla_t}}{mT}}\Jmax \leq \frac{\tilde{C}\V\log{T}}{mT} + \frac{\norm{\nabla_t}\log{T}}{mT}\; ,
    \end{align*}
    where the last inequality holds as $10\sqrt{\log\brac{16m^2T}}\leq \tilde{C}$.
\end{proof}

\begin{lemma}\label{lem:2nd_order_aggr_mfm}
    Consider $\widehat{g}_t^{j}$ defined in \Cref{eq:mfm_aggregated_grad}. For every $j=0,\ldots,\Jmax\coloneqq\floor{\log{T}}$,
    \[
        \E\lVert{\widehat{g}_t^{j} - \nabla_t}\rVert^2 \leq \frac{2\tilde{C}^2\V^2\tilde{\gamma}}{2^j} + \frac{\E\norm{\nabla_t}^2}{4mT}\; .
    \]
\end{lemma}
\begin{proof}
    Again, closely following the steps in the proof of \Cref{lem:2nd_order_aggr}, replacing \Cref{lem:core_lemma} with \Cref{lem:mfm}. By item 2 of \Cref{lem:mfm}, it holds with probability at least $1-\nicefrac{1}{4mT}$ that 
    \[
        \lVert{\widehat{g}_t^{j} - \nabla_t}\rVert^2 \leq \frac{\tilde{C}^2\V^2\tilde{\gamma}}{2^j}\; .
    \]
    In addition, item 1 of \Cref{lem:mfm} implies that $\lVert{\widehat{g}_t^{j} - \nabla_t\rVert}^2 \leq 100\log\brac{16m^2 T}\V^2 + \norm{\nabla_t}^2$, deterministically. Combining these results, by the law of total expectation, we have 
    \begin{align*}
        \E\lVert{\widehat{g}_t^{j} - \nabla_t}\rVert^2 &\leq \frac{\tilde{C}^2 \V^2 \tilde{\gamma}}{2^j} + \brac{100\log\brac{16m^2 T}\V^2 + \E\norm{\nabla_t}^2}\cdot\frac{1}{4mT} \\ &\leq \frac{\tilde{C}^2 \V^2 \tilde{\gamma}}{2^j} + \frac{\tilde{C}^2\V^2}{mT} + \frac{\E\norm{\nabla_t}^2}{4mT} \\ &\leq \frac{2\tilde{C}^2 \V^2 \tilde{\gamma}}{2^j} + \frac{\E\norm{\nabla_t}^2}{4mT}\; ,
        % \frac{C^2 \V^2 \gamma}{2^{j}} + \frac{4C^2 \V^2 \gamma}{2^j} = \frac{5C^2 \V^2 \gamma}{2^j}\; ,
    \end{align*}
    where second inequality stems from $25\log\brac{16m^2 T}\leq\tilde{C}^2$, and the final inequality results from $\nicefrac{1}{m}\leq\tilde{\gamma}$ and $2^{j}\leq T$, which holds for every $j=0,\ldots,\floor{\log{T}}$.
\end{proof}

\begin{lemma}[MLMC Variance -- MFM]\label{lem:mlmc_2nd_mfm}
    Consider the MLMC gradient estimator in \Cref{eq:mlmc_agg_mfm}. For every $t\in\sbrac{T}$:
    \begin{equation*}
        \E\norm{g_t - \nabla_t}^2 \leq \begin{cases}
            23\tilde{C}^2\V^2\log{T} + \frac{\E\norm{\nabla_t}^2}{2mT}, &t\in\badrounds \\
            28\tilde{C}^2 \V^2 \tilde{\gamma} \log{T} + 4\log{T}\E\norm{\nabla_t}^2, &t\notin\badrounds
        \end{cases}\; .
    \end{equation*}
\end{lemma}
\begin{proof}
    The proof aligns with the approach used in the proof of \Cref{lem:mlmc_2nd_general}, with minor adjustments that leverage \Cref{lem:2nd_order_aggr_mfm}. Additionally, it introduces a distinct bound on $\E\lVert g_t - \nabla_t\rVert^2$ based on whether the round $t$ is good or bad. By taking expectation w.r.t $J_t$, we obtain \Cref{eq:mlmc_second_moment_explicit}, namely,
    \begin{align*}
        \E\norm{g_t - \nabla_t}^2 &\leq 2\E\norm{\widehat{g}_t^{0} - \nabla_t}^2 + 2\sum_{j=1}^{\Jmax}{2^{j}\underbrace{\E\sbrac{\lVert{\widehat{g}_t^{j} - \widehat{g}_t^{j-1}}\rVert^2\mathbbm{1}_{\Ecal_t(j)}}}_{=(\dag)}}\; .
    \end{align*}
    We bound $(\dag)$ differently for $t\in\badrounds$ and $t\notin\badrounds$. Starting with $t\in\badrounds$, it holds that
    \begin{align*}
        \E\sbrac{\lVert{\widehat{g}_t^{j} - \widehat{g}_t^{j-1}}\rVert^2\mathbbm{1}_{\Ecal_t(j)}} &= \E\sbrac{\lVert{\widehat{g}_t^{j} - \widehat{g}_t^{j-1}}\rVert^2 | \Ecal_t(j)}\underbrace{\prob(\Ecal_t(j))}_{\leq 1} \leq \frac{9\tilde{C}^2\V^2}{2^{j}}\; ,
    \end{align*}
    where in the final inequality, we utilize the constraint on $\lVert{ \widehat{g}_t^{j} - \widehat{g}_t^{j-1}\rVert}$, conditioned on the event $\Ecal_t (j)$ (refer to \Cref{eq:event_E_option2}). Proceeding to $t\notin\badrounds$, \Cref{lem:2nd_order_aggr_mfm} implies that
    \begin{align*}
        \E\sbrac{\lVert{\widehat{g}_t^{j} - \widehat{g}_t^{j-1}}\rVert^2\mathbbm{1}_{\Ecal_t(j)}} \leq \E\lVert{\widehat{g}_t^{j} - \widehat{g}_t^{j-1}}\rVert^2 &\leq 2\E\lVert{\widehat{g}_t^{j} - \nabla_t}\rVert^2 + 2\E\lVert{\widehat{g}_t^{j-1} - \nabla_t}\rVert^2 \\ &\leq 2\brac{\frac{2\tilde{C}^2\V^2\tilde{\gamma}}{2^j} + \frac{\E\norm{\nabla_t}^2}{4mT}} + 2\brac{\frac{2\tilde{C}^2\V^2\tilde{\gamma}}{2^{j-1}} + \frac{\E\norm{\nabla_t}^2}{4mT}} \\ &= \frac{12\tilde{C}^2 \V^2\tilde{\gamma}}{2^{j}} + \frac{\E\norm{\nabla_t}^2}{mT} \\ &\leq \frac{12\tilde{C}^2 \V^2\tilde{\gamma} + \E\norm{\nabla_t}^2}{2^{j}}\; ,
        % 4\brac{\frac{3\tilde{C}^2\V^2\tilde{\gamma}}{2^{j}} + \frac{\E\norm{\nabla_t}^2}{mT}} \\ &\leq \frac{4}{2^{j}}\brac{3\tilde{C}^2\V^2\tilde{\gamma} + \frac{\E\norm{\nabla_t}^2}{m}}\; ,
    \end{align*}
    where the last inequality follows from $2^{j}\leq T$ and $m\geq 1$. We can thus conclude that
    \begin{align*}
        \E\sbrac{\lVert{\widehat{g}_t^{j} - \widehat{g}_t^{j-1}}\rVert^2\mathbbm{1}_{\Ecal_t(j)}} \leq \begin{cases}
            9\tilde{C}^2\V^2 / 2^{j}, & t\in\badrounds \\
            (12\tilde{C}^2 \V^2\tilde{\gamma} + \E\norm{\nabla_t}^2) / 2^{j}, &t\notin\badrounds
        \end{cases}\; .
    \end{align*}
    In addition, \Cref{lem:2nd_order_aggr_mfm} implies that $\E\lVert \widehat{g}_t^{0}-\nabla_t \rVert^2\leq 2\tilde{C}^2 \V^2\tilde{\gamma} + \nicefrac{\norm{\nabla_t}^2}{4mT}$. Plugging these bounds back into \Cref{eq:mlmc_second_moment_explicit} concludes the proof. Specifically, for $t\in\badrounds$,
    \begin{align*}
        \E\norm{g_t - \nabla_t}^2 &\leq 2\brac{2\tilde{C}^2 \V^2\tilde{\gamma} + \frac{\E\norm{\nabla_t}^2}{4mT}} + 2\sum_{j=1}^{\Jmax}{2^{j}\cdot\frac{9\tilde{C}^2\V^2}{2^{j}}} \\ &= 4\tilde{C}^2 \V^2\tilde{\gamma} + \frac{\E\norm{\nabla_t}^2}{2mT} + 18\tilde{C}^2 \V^2 \Jmax \\ &\leq 23\tilde{C}^2\V^2\log{T} + \frac{\E\norm{\nabla_t}^2}{2mT}\; ,
    \end{align*}
    where the last inequality holds as $4\tilde{\gamma}\leq 5$ and $1\leq\Jmax\leq\log{T}$. 
    On the other hand, for $t\notin\badrounds$, it holds that 
    \begin{align*}
        \E\norm{g_t - \nabla_t}^2 &\leq 2\brac{2\tilde{C}^2 \V^2\tilde{\gamma} + \frac{\E\norm{\nabla_t}^2}{4mT}} + 2\sum_{j=1}^{\Jmax}{2^{j}\cdot\frac{12\tilde{C}^2 \V^2\tilde{\gamma} + \E\norm{\nabla_t}^2}{2^{j}}} \\ &\leq 4\tilde{C}^2 \V^2\tilde{\gamma} + \frac{2\E\norm{\nabla_t}^2}{mT} + 24\tilde{C}^2\V^2\tilde{\gamma}\Jmax + 2\Jmax\E\norm{\nabla_t}^2 \\ &\leq 28\tilde{C}^2 \V^2 \tilde{\gamma} \log{T} + 4\log{T}\E\norm{\nabla_t}^2\; .
    \end{align*}
\end{proof}

\subsection{Proof of \Cref{thm:convex-adaptive}}\label{subapp:convex-mfm}
To prove \Cref{thm:convex-adaptive}, we present a lemma that establishes a regret bound for AdaGrad~\cite{levy2017online}, crucial for our analysis. We provide the proof for completeness.
\begin{lemma}\label{lem:adagrad_regret_bound}
    Consider the AdaGrad update rule, namely, \Cref{eq:adagrad_update}, and suppose \Cref{assump:bounded-domain} holds, i.e., the domain $\K$ is bounded with diameter $D\coloneqq \max_{x,y\in\K}{\norm{x-y}}$. Then, for every $u\in\K$, the iterates $x_1,\ldots,x_T$ satisfy:
    \[
        \sum_{t=1}^{T}{g_t^\top(x_t - u)} \leq \brac{\frac{D^2}{2\eta_0} + \eta_0}\sqrt{\sum_{t=1}^{T}{\norm{g_{t}}^2}}\; .
    \]
\end{lemma}
\begin{proof}
    Our proof follows that of Theorem 1.1 in \citep{levy2017online}. For every $u\in\K$, we have that
    \begin{align*}
        \norm{x_{t+1} - u}^2 &\leq \norm{x_{t} - u}^2 - 2\eta_t g_t^\top (x_t - u) + \eta^2\norm{g_t}^2\; .
    \end{align*}
    Rearranging terms, we get:
    \begin{align*}
        g_t^\top(x_t - u) &\leq \frac{\norm{x_t - u}^2 - \norm{x_{t+1} - u}^2}{2\eta_t} + \frac{\eta_t}{2}\norm{g_t}^2\; .
    \end{align*}
    Summing over $t\in\sbrac{T}$, we then obtain:
    \begin{align*}
        \sum_{t=1}^{T}{g_t^\top(x_t - u)} &\leq \frac{\norm{x_1 -u}^2}{2\eta_1} + \sum_{t=2}^{T}{\frac{\norm{x_t - u}^2}{2}\brac{\frac{1}{\eta_t} - \frac{1}{\eta_{t-1}}}} + \frac{1}{2}\sum_{t=1}^{T}{\eta_t \norm{g_t}^2} \\ &\leq \frac{D^2}{2}\brac{\frac{1}{\eta_1} + \sum_{t=2}^{T}{\brac{\frac{1}{\eta_t} - \frac{1}{\eta_{t-1}}}}} + \frac{\eta_0}{2}\sum_{t=1}^{T}{\frac{\norm{g_t}^2}{\sqrt{\sum_{s=1}^{t}{\norm{g_{s}}^2}}}} \\ &= \frac{D^2}{2\eta_T} + \frac{\eta_0}{2}\sum_{t=1}^{T}{\frac{\norm{g_t}^2}{\sqrt{\sum_{s=1}^{t}{\norm{g_s}^2}}}} \\ &\leq \frac{D^2}{2\eta_0}\sqrt{\sum_{t=1}^{T}{\norm{g_t}^2}} + \eta_0\sqrt{\sum_{t=1}^{T}{\norm{g_t}^2}} \\ &=\brac{\frac{D^2}{2\eta_0} + \eta_0}\sqrt{\sum_{t=1}^{T}{\norm{g_{t}}^2}}\; ,
    \end{align*}
    where the second inequality uses $\norm{x_t - u}^2\leq D^2$ for every $t\in\sbrac{T}$ and $\eta_t\leq \eta_{t-1}$, and the final inequality stems from \Cref{lem:sum_sqrt_lemma}.
\end{proof}

We continue to prove \Cref{thm:convex-adaptive}, presented again here for ease of use.
\convexadaptive*

\begin{proof}
    Denote: $R_T=\sum_{t\in\sbrac{T}}{f(x_t) - f^*}$. By the convexity of $f$,
    \begin{align}\label{eq:bias-var-decomp-adaptive}
         \E[R_T] \leq \E\sbrac{\sum_{t\in\sbrac{T}}{\nabla_t^\top(x_t - x^*)}} = \underbrace{\E\sbrac{\sum_{t\in\sbrac{T}}{g_t^{\top}(x_t - x^*)}}}_{=(A)} + \underbrace{\E\sbrac{\sum_{t\in\sbrac{T}}{\brac{\nabla_t - g_t}^\top(x_t - x^*)}}}_{=(B)}\; .
    \end{align}
    \paragraph{Bounding $(A)$. } Utilizing AdaGrad's regret bound, namely \Cref{lem:adagrad_regret_bound}, with $\eta_0 = \nicefrac{D}{\sqrt{2}}$, we obtain:
    \begin{align*}
        \sum_{t\in\sbrac{T}}{g_t^{\top}(x_t - x^*)} \leq D\sqrt{2\sum_{t\in\sbrac{T}}{\norm{g_t}^2}} &\leq 2D\sqrt{\sum_{t\in\sbrac{T}}{\norm{g_t - \nabla_t}^2}} + 2D\sqrt{\sum_{t\in\sbrac{T}}{\norm{\nabla_t}^2}}\; .
    \end{align*}
    Taking expectation and using applying Jensen's inequality yields:
    \begin{align*}
        \E\!\sum_{t\in\sbrac{T}}{g_t^{\top}(x_t - x^*)} &{\leq} 2D\E\!\sqrt{\sum_{t\in\sbrac{T}}{\norm{g_t - \nabla_t}^2}} + 2D\E\!\sqrt{\sum_{t\in\sbrac{T}}{\norm{\nabla_t}^2}} \leq 2D\sqrt{\sum_{t\in\sbrac{T}}{\E\!\norm{g_t - \nabla_t}^2}} + 2D\sqrt{\sum_{t\in\sbrac{T}}{\E\!\norm{\nabla_t}^2}}\; .
    \end{align*}
    \paragraph{Bounding $(B)$. } We proceed with the same steps employed to derive the bound on $(\star)$ in the proof of \Cref{thm:convex}, replacing \Cref{lem:mlmc_1st_general,lem:2nd_order_aggr,lem:mlmc_2nd_general} with \Cref{lem:mlmc_1st_mfm,lem:mlmc_2nd_mfm}, respectively. Specifically, we have 
    \begin{align*}
        \E\sbrac{\sum_{t\in\sbrac{T}}{\brac{\nabla_t - g_t}^\top(x_t - x^*)}} &\!\leq\! D\sqrt{\abs{\badrounds}}\sqrt{\sum_{t\in\badrounds}{\E\norm{g_t - \nabla_t}^2}} + D\sqrt{T}\sqrt{\sum_{t\notin\badrounds}{\E\lVert \widehat{g}_t^{\Jmax} - \nabla_t\rVert^2}} + D\sqrt{T}\sqrt{\sum_{t\notin\badrounds}{\E\norm{y_t}^2}}\; ,
    \end{align*}
    where, according to \Cref{lem:mlmc_1st_mfm,lem:2nd_order_aggr_mfm} (and $2^{\Jmax}\geq\nicefrac{T}{2}$),
    \begin{equation}\label{eq:jmax_and_yt_mfm}
        \E\lVert{\widehat{g}_t^{\Jmax} - \nabla_t}\rVert^2 \leq \frac{4\tilde{C}^2\V^2\tilde{\gamma}}{T} + \frac{\E\norm{\nabla_t}^2}{4mT}, \quad\text{ and }\quad \norm{y_t}^2 \leq \frac{2\log^2{T}(\tilde{C}^2\V^2 + \lVert{\nabla_t}\rVert^2)}{m^2T^2}\; .
    \end{equation}
    Plugging the bounds on $(A)$ and $(B)$ back into \Cref{eq:bias-var-decomp-adaptive} gives:
    \begin{align*}
        \E[R_T] &\leq 2D\sqrt{\sum_{t\in\sbrac{T}}{\E\norm{g_t - \nabla_t}^2}} + 2D\sqrt{\sum_{t\in\sbrac{T}}{\E\norm{\nabla_t}^2}} + D\sqrt{\abs{\badrounds}}\sqrt{\sum_{t\in\badrounds}{\E\norm{g_t - \nabla_t}^2}} \nonumber \\ &\quad+ D\sqrt{T}\sqrt{\sum_{t\notin\badrounds}{\E\lVert \widehat{g}_t^{\Jmax} - \nabla_t\rVert^2}} + D\sqrt{T}\sqrt{\sum_{t\notin\badrounds}{\E\norm{y_t}^2}}\; .
    \end{align*}
    Employing the bounds on $\E\lVert{\widehat{g}_t^{\Jmax} - \nabla_t}\rVert^2$ and $\norm{y_t}^2$ (\Cref{eq:jmax_and_yt_mfm}) in conjunction with \Cref{lem:mlmc_2nd_mfm} and some algebra, we get that
    \begin{align*}
        \E[R_T] &\leq 2D\sqrt{\sum_{t\in\badrounds}{\brac{23\tilde{C}^2\V^2\log{T} + \frac{\E\norm{\nabla_t}^2}{2mT}}} + \sum_{t\notin\badrounds}{\brac{28\tilde{C}^2\V^2\tilde{\gamma}\log{T} + 4\log{T}\E\norm{\nabla_t}^2}}} \\ &\quad+ 2D\sqrt{\sum_{t\in\sbrac{T}}{\E\norm{\nabla_t}^2}} + D\sqrt{\abs{\badrounds}}\sqrt{\sum_{t\in\badrounds}{\brac{23\tilde{C}^2\V^2\log{T} + \frac{\E\norm{\nabla_t}^2}{2mT}}}} \\ &\quad+ D\sqrt{T}\sqrt{\sum_{t\notin\badrounds}{\brac{\frac{4\tilde{C}^2 \V^2 \tilde{\gamma}}{T} + \frac{\E\norm{\nabla_t}^2}{4mT}}}} + D\sqrt{T}\sqrt{\sum_{t\notin\badrounds}{\frac{2\log^2{T}(\tilde{C}^2\V^2 + \E\lVert{\nabla_t}\rVert^2)}{m^2T^2}}} \\ &\leq \underbrace{2\sqrt{23}\tilde{C}D\V\sqrt{\abs{\badrounds}\log{T}}}_{=(A)} + \underbrace{2\sqrt{28}\tilde{C}D\V\sqrt{\tilde{\gamma}T\log{T}}}_{=(B)} + \underbrace{4D\sqrt{\log{T}\sum_{t\in\sbrac{T}}{\norm{\nabla_t}^2}}}_{=(C)} \\ &\quad+ \underbrace{2D\sqrt{\sum_{t\in\sbrac{T}}{\E\norm{\nabla_t}^2}}}_{=(D)} + \underbrace{\sqrt{23}\tilde{C}D\V\abs{\badrounds}\sqrt{\log{T}}}_{=(E)} + \underbrace{D\sqrt{\frac{\abs{\badrounds}}{2mT}\sum_{t\in\sbrac{T}}{\E\norm{\nabla_t}^2}}}_{=(F)} \\ &\quad+ \underbrace{2\tilde{C}D\V\sqrt{\tilde{\gamma}T}}_{=(G)} + \underbrace{D\sqrt{\frac{1}{4m}\sum_{t\in\sbrac{T}}{\E\norm{\nabla_t}^2}}}_{=(H)} + \underbrace{\sqrt{2}\tilde{C}D\V\frac{\log{T}}{m}}_{=(I)} + \underbrace{D\sqrt{\frac{2\log^2{T}}{m^2 T}\sum_{t\in\sbrac{T}}{\E\norm{\nabla_t}^2}}}_{=(J)}\; .
    \end{align*}
    Note that we can bound
    \[
        (A) + (E) = 2\sqrt{23}\tilde{C}D\V\sqrt{\abs{\badrounds}\log{T}} + \sqrt{23}\tilde{C}D\V\abs{\badrounds}\sqrt{\log{T}} \leq 15\tilde{C}D\V\abs{\badrounds}\sqrt{\log{T}}\; .
    \]
    In addition, we have
    \begin{align*}
        (B) + (G) &= 2\sqrt{28}\tilde{C}D\V\sqrt{\tilde{\gamma}T\log{T}} + 2\tilde{C}D\V\sqrt{\tilde{\gamma}T} \leq 13\tilde{C}D\V\sqrt{\tilde{\gamma}T\log{T}}\; .
    \end{align*}
    It also holds that 
    \begin{align*}
        (C) + (D) + (F) + (H) + (J) &= \brac{4\sqrt{\log{T}} + 2 + \sqrt{\frac{\abs{\badrounds}}{2mT}} + \frac{1}{2\sqrt{m}} + \frac{\sqrt{2}\log{T}}{m\sqrt{T}}}D\sqrt{\sum_{t\in\sbrac{T}}{\E\norm{\nabla_t}^2}} \\ &\leq \brac{4\sqrt{\log{T}} + 2 + \frac{1}{\sqrt{2}m} + \frac{1}{2\sqrt{m}} + \frac{\sqrt{2}}{m}}D\sqrt{\sum_{t\in\sbrac{T}}{\E\norm{\nabla_t}^2}} \\ &\leq 9D\sqrt{\log{T}\sum_{t\in\sbrac{T}}{\E\norm{\nabla_t}^2}}\; ,
    \end{align*}
    where the second inequality holds as $\log{T}\leq\sqrt{T}$ for every $T\in\mathbb{N}$ and $\abs{\badrounds}\leq T$; and the last inequality follows from $m\geq 1$ and $\frac{1}{\sqrt{2}} + \frac{1}{2} + \sqrt{2}\leq 3$. Injecting these bounds back, we obtain:
    \begin{align*}
        \E[R_T] &\leq 15\tilde{C}D\V\abs{\badrounds}\sqrt{\log{T}} + 13\tilde{C}D\V\sqrt{\tilde{\gamma}T\log{T}} + \sqrt{2}\tilde{C}D\V\frac{\log{T}}{m} + 9D\sqrt{\log{T}\sum_{t\in\sbrac{T}}{\E\norm{\nabla_t}^2}} \\ &\leq 15\tilde{C}D\V\abs{\badrounds}\sqrt{\log{T}} + 13\tilde{C}D\V\sqrt{\tilde{\gamma}T\log{T}} + \sqrt{2}\tilde{C}D\V\tilde{\gamma}\log{T} + 9D\sqrt{2L\log{T}\E[R_T]}\; ,
    \end{align*}
    where the final inequality stems from $\nicefrac{1}{m}\leq\tilde{\gamma}$ and from \Cref{lem:self_boundness}, which implies that $\sum_{t\in\sbrac{T}}{\norm{\nabla_t}^2}\leq 2L R_T$. By applying \Cref{lem:simple_cases_lemma} with $a=\E[R_T]$, $b=15\tilde{C}D\V\abs{\badrounds}\sqrt{\log{T}} + 13\tilde{C}D\V\sqrt{\tilde{\gamma}T\log{T}} + \sqrt{2}\tilde{C}D\V\tilde{\gamma}\log{T}$, $c=9D$, and $d=2L\log{T}$, we get
    \begin{align*}
        \E[R_T] &\leq 30\tilde{C}D\V\abs{\badrounds}\sqrt{\log{T}} + 26\tilde{C}D\V\sqrt{\tilde{\gamma}T\log{T}} + 2\sqrt{2}\tilde{C}D\V\tilde{\gamma}\log{T} + 648LD^2\log{T}\; .
    \end{align*}
    Dividing by $T$ and employing Jensen's inequality finally gives:
    \begin{align*}
        \E[f(\widebar{x}_T - f^*)] \leq \frac{\E[R_T]}{T} \leq 26\tilde{C}D\V\sqrt{\frac{\tilde{\gamma}\log{T}}{T}} + 30\tilde{C}D\V\frac{\abs{\badrounds}\sqrt{\log{T}}}{T} + 2\sqrt{2}\tilde{C}D\V\frac{\tilde{\gamma}\log{T}}{T} + 648LD^2\frac{\log{T}}{T}\; .
    \end{align*}
\end{proof}

\subsection{Proof of \Cref{thm:nonconvex-adaptive}}\label{subapp:nonconvex-mfm}
The following lemma provides an upper bound on the sum of squared gradient norms when utilizing AdaGrad for smooth and bounded functions, which we use to prove \Cref{thm:nonconvex-adaptive}.
\begin{lemma}\label{lem:adagrad_sum_of_grad_norms_smooth_func}
    Consider the AdaGrad update rule, namely, \Cref{eq:adagrad_update}, with $\K=\reals^{d}$. Suppose \Cref{assump:smooth} holds and assume that $f$ is bounded by $M$, i.e., $\max_{x}{\abs{f(x)}}\leq M$. Then, the iterates $x_1,\ldots,x_T$ satisfy:
    \begin{equation*}
        \sum_{t=1}^{T}{\norm{\nabla_t}^2} \leq \brac{\frac{2M}{\eta_0} + \eta_0 L}\sqrt{\sum_{t=1}^{T}{\lVert g_t\rVert}^2} + \sum_{t=1}^{T}{\brac{\nabla_t - g_t}^\top\nabla_t}\; .
    \end{equation*}
\end{lemma}
\begin{proof}
    By the smoothness of $f$, for every $x,y\in\reals^d$ we have that $f(y)\leq f(x) + \nabla f(x)^\top(y-x) + \frac{L}{2}\norm{y-x}^2$. Plugging-in the update rule $x_{t+1} = x_t - \eta_t g_t$, we obtain:
    \begin{align*}
        f(x_{t+1}) &\leq f(x_t) - \eta_t \nabla_t^\top g_t + \frac{L\eta_t^2}{2}\norm{g_t}^2 \\ &= f(x_t) - \eta_t \norm{\nabla_t}^2 + \eta_t \brac{\nabla_t - g_t}^\top\nabla_t + \frac{L\eta_t^2}{2}\norm{g_t}^2\; .
    \end{align*}
    Rearranging terms and dividing by $\eta_t$ gives:
    \begin{equation*}
        \norm{\nabla_t}^2 \leq \frac{f(x_t) - f(x_{t+1})}{\eta_t} + \frac{L\eta_t}{2}\norm{g_t}^2 + \brac{\nabla_t - g_t}^\top\nabla_t\; .
    \end{equation*}
    Denote: $\Delta_t = f(x_t) - f^*$, and $\Delta_{\max} = \max_{t\in\sbrac{T}}{f(x_t) - f^*}$. Thus, the above is equivalent to  
    \begin{equation*}
        \norm{\nabla_t}^2 \leq \frac{\Delta_t - \Delta_{t+1}}{\eta_t} + \frac{L\eta_t}{2}\norm{g_t}^2 + \brac{\nabla_t - g_t}^\top\nabla_t\; .
    \end{equation*}
    Summing over $t=1,\ldots,T$, we obtain that 
    \begin{align}\label{eq:lem_helper}
        \sum_{t\in\sbrac{T}}{\norm{\nabla_t}^2} &\leq \sum_{t\in\sbrac{T}}{\frac{\Delta_t - \Delta_{t+1}}{\eta_t}} + \frac{L}{2}\sum_{t\in\sbrac{T}}{\eta_t\norm{g_t}^2} + \sum_{t\in\sbrac{T}}{\brac{\nabla_t - g_t}^\top\nabla_t} \nonumber \\ &\leq \frac{\Delta_{\max}}{\eta_T} + \frac{L}{2}\sum_{t\in\sbrac{T}}{\eta_t\norm{g_t}^2} + \sum_{t\in\sbrac{T}}{\brac{\nabla_t - g_t}^\top\nabla_t} \; ,
    \end{align}
    where the last inequality follows from:
    \begin{equation*}
        \sum_{t=1}^{T}{\frac{\Delta_t - \Delta_{t+1}}{\eta_t}} = \frac{\Delta_1}{\eta_1} + \sum_{t=2}^{T}{\brac{\frac{1}{\eta_t} - \frac{1}{\eta_{t-1}}}\Delta_t} - \frac{\Delta_{T+1}}{\eta_{T}} \leq \frac{\Delta_1}{\eta_1} + \sum_{t=2}^{T}{\brac{\frac{1}{\eta_t} - \frac{1}{\eta_{t-1}}}\Delta_t} \leq \frac{\Delta_{\max}}{\eta_T}\; ,
    \end{equation*}
    which holds as $\eta_{t} = \eta_0(\sum_{\tau=1}^{t}{\norm{g_{\tau}}^2})^{-1/2}$ is non-increasing. Next, we can bound the second term in the R.H.S of \Cref{eq:lem_helper} using \Cref{lem:sum_sqrt_lemma} with $a_i = \lVert g_i\rVert^2$ as follows: 
    \begin{align*}
        \sum_{t\in\sbrac{T}}{\eta_t \norm{g_t}^2} &= \eta_0\sum_{t\in\sbrac{T}}{\frac{\norm{g_t}^2}{\sqrt{\sum_{s=1}^{t}{\norm{g_{s}}^2}}}} \leq 2\eta_0\sqrt{\sum_{t\in\sbrac{T}}{\norm{g_t}^2}}\; .
    \end{align*}
    Injecting this bound and $\eta_T$ back into \Cref{eq:lem_helper} and considering that $\Delta_{\max}\leq 2M$ concludes the proof.
\end{proof}

Next, we prove \Cref{thm:nonconvex-adaptive}, recapitulated here for easy access.
\nonconvexadaptive*
\begin{proof}
    Denote: $R_T = \sum_{t\in\sbrac{T}}{\norm{\nabla_t}^2}$. Using \Cref{lem:adagrad_sum_of_grad_norms_smooth_func} and Jensen's inequality, we have that 
    \begin{align}\label{eq:main_eq_nonconvex}
        \E[R_T] &\leq \E\sbrac{F\sqrt{\sum_{t\in\sbrac{T}}{\lVert g_t\rVert}^2}} + \sum_{t\in\sbrac{T}}{\E\sbrac{\brac{\nabla_t - g_t}^\top\nabla_t}} \nonumber \\ &\leq F\sqrt{\sum_{t\in\sbrac{T}}{\E\lVert g_t\rVert}^2} + \sum_{t\in\sbrac{T}}{\E\sbrac{\brac{\nabla_t - g_t}^\top\nabla_t}} \nonumber \\ &\leq F\sqrt{2\sum_{t\in\sbrac{T}}{\E\lVert g_t - \nabla_t\rVert}^2} + F\sqrt{2\E[R_T]} + \underbrace{\sum_{t\in\sbrac{T}}{\E\sbrac{\brac{\nabla_t - g_t}^\top\nabla_t}}}_{=(\star)}\; .
    \end{align} 
    We follow the same steps used to establish the bound on $(\star)$ in the proof of \Cref{thm:nonconvex}, substituting \Cref{lem:mlmc_1st_general,lem:2nd_order_aggr,lem:mlmc_2nd_general} with \Cref{lem:mlmc_1st_mfm,lem:2nd_order_aggr_mfm,lem:mlmc_2nd_mfm}, respectively. Concretely, we obtain \Cref{eq:bound_on_star}, 
    \begin{align*}
        \sum_{t\in\sbrac{T}}{\E\sbrac{\brac{\nabla_t - g_t}^\top\nabla_t}} &\leq \frac{1}{2}\sum_{t\in\badrounds}{\E\norm{g_t - \nabla_t}^2} + \sum_{t\notin\badrounds}{\brac{\E\lVert\widehat{g}_t^{\Jmax} - \nabla_t\rVert^2 + \E\lVert{y_t}\rVert^2}} + \frac{1}{2}\E[R_T]\; ,
    \end{align*}
    where, according to \Cref{lem:mlmc_1st_mfm,lem:2nd_order_aggr_mfm},
    \[
        \E\lVert{\widehat{g}_t^{\Jmax} - \nabla_t}\rVert^2 \leq \frac{4\tilde{C}^2\V^2\tilde{\gamma}}{T} + \frac{\E\norm{\nabla_t}^2}{4mT}, \quad\text{ and }\quad \norm{y_t}^2 \leq \frac{2\log^2{T}(\tilde{C}^2\V^2 + \lVert{\nabla_t}\rVert^2)}{m^2T^2}\; .
    \]
    Plugging \Cref{eq:bound_on_star} back into \Cref{eq:main_eq_nonconvex} yields:
    \begin{align*}
        \E[R_T] &\!\leq\! F\sqrt{2\sum_{t\in\sbrac{T}}{\E\lVert g_t - \nabla_t\rVert}^2} + F\sqrt{2\E[R_T]} + \frac{1}{2}\sum_{t\in\badrounds}{\E\norm{g_t - \nabla_t}^2} + \sum_{t\notin\badrounds}{\brac{\E\lVert\widehat{g}_t^{\Jmax} - \nabla_t\rVert^2 + \E\lVert{y_t}\rVert^2}} {+} \frac{1}{2}\E[R_T]\; .
    \end{align*}
    Subtracting $\frac{1}{2}\E[R_T]$ and multiplying by $2$ gives:
    \begin{align*}
        \E[R_T] &\leq 2\sqrt{2}F\sqrt{\sum_{t\in\sbrac{T}}{\E\lVert g_t - \nabla_t\rVert}^2} + 2F\sqrt{2\E[R_T]} + \sum_{t\in\badrounds}{\E\norm{g_t - \nabla_t}^2} + 2\sum_{t\notin\badrounds}{\E\lVert\widehat{g}_t^{\Jmax} - \nabla_t\rVert^2} + 2\sum_{t\notin\badrounds}{\E\lVert{y_t}\rVert^2}\; .
    \end{align*}
    Substituting the bounds on $\E\lVert{\widehat{g}_t^{\Jmax} - \nabla_t}\rVert^2$, $\norm{y_t}^2$, and $\E\norm{g_t - \nabla_t}^2$ (\Cref{lem:mlmc_2nd_mfm}), we obtain
    \begin{align*}
        \E[R_T] &\leq 2\sqrt{2}F\sqrt{\sum_{t\in\badrounds}{\brac{23\tilde{C}^2\V^2\log{T} + \frac{\E\norm{\nabla_t}^2}{2mT}}} + \sum_{t\notin\badrounds}{\brac{28\tilde{C}^2\V^2\tilde{\gamma}\log{T} + 4\log{T}\E\norm{\nabla_t}^2}}} \\ &\quad+2F\sqrt{2\E[R_T]} + \sum_{t\in\badrounds}{\brac{23\tilde{C}^2\V^2\log{T} + \frac{\E\norm{\nabla_t}^2}{2mT}}} + 2\sum_{t\notin\badrounds}{\brac{\frac{4\tilde{C}^2\V^2\tilde{\gamma}}{T} + \frac{\E\norm{\nabla_t}^2}{4mT}}} \\ &\quad+ 2\sum_{t\notin\badrounds}{\frac{2\log^2{T}(\tilde{C}^2\V^2 + \E\lVert{\nabla_t}\rVert^2)}{m^2T^2}} \\ &\leq \underbrace{2\sqrt{46}\tilde{C}F\V\sqrt{\abs{\badrounds}\log{T}}}_{=(A)} + 2\sqrt{56}\tilde{C}F\V\sqrt{\tilde{\gamma}T\log{T}} + \underbrace{4F\sqrt{\log{T}\E[R_T]}}_{=(B)} \\ &\quad+\underbrace{2F\sqrt{2\E[R_T]}}_{=(C)} + \underbrace{23\tilde{C}^2\V^2\abs{\badrounds}\log{T}}_{=(D)} + 8\tilde{C}^2\V^2\tilde{\gamma} + \underbrace{\frac{1}{2mT}\E[R_T]}_{=(E)} \\&\quad +\frac{4\tilde{C}^2 \V^2\log^2{T}}{m^2 T} + \underbrace{\frac{4\log^2{T}}{m^2 T^2}\E[R_T]}_{=(F)}\; .
    \end{align*}
    We can bound the sum of $(A)$ and $(D)$ as,
    \begin{align*}
        (A) + (D) &= 2\sqrt{46}\tilde{C}F\V\sqrt{\abs{\badrounds}\log{T}} + 23\tilde{C}^2\V^2\abs{\badrounds}\log{T} \leq 23\tilde{C}\V(F + \tilde{C}\V)\abs{\badrounds}\log{T}\; .
    \end{align*}
    In addition, we have,
    \begin{align*}
        (B) + (C) &= \brac{4\sqrt{\log{T}} + 2\sqrt{2}}F\sqrt{\E[R_T]} \leq 7F\sqrt{\log{T}\E[R_T]}\; .
    \end{align*}
    Furthermore, we can also bound the sum of $(E)$ and $(F)$ as follows:
    \begin{align*}
        (E) + (F) &= \brac{\frac{1}{2mT} + \frac{4\log^2{T}}{m^2 T^2}}\E[R_T] \leq \brac{\frac{1}{2T} + \frac{4\log^2{T}}{T^2}}\E[R_T] \leq \frac{1}{2}\E[R_T]\; ,
    \end{align*}
    where the final inequality holds as $\nicefrac{1}{2T}\leq\nicefrac{1}{4}$ and $\nicefrac{4\log^2{T}}{T^2}\leq\nicefrac{1}{4}$ for every $T\geq 2$. Plugging these bound back, we get that
    \begin{align*}
        \E[R_T] &\!\leq\! 23\tilde{C}\V(F + \tilde{C}\V)\abs{\badrounds}\log{T} + 2\sqrt{56}\tilde{C}F\V\sqrt{\tilde{\gamma}T\log{T}} \!+\! 7F\sqrt{\log{T}\E[R_T]} + 8\tilde{C}^2\V^2\tilde{\gamma} + \frac{4\tilde{C}^2 \V^2\log^2{T}}{m^2 T} \!+\! \frac{\E[R_T]}{2}\; .
    \end{align*}
    Subtracting $\frac{1}{2}\E[R_T]$ and then multiplying by $2$ gives:
    \begin{align*}
        \E[R_T] &\leq 46\tilde{C}\V(F + \tilde{C}\V)\abs{\badrounds}\log{T} + 4\sqrt{56}\tilde{C}F\V\sqrt{\tilde{\gamma}T\log{T}} + 16\tilde{C}^2 \V^2\tilde{\gamma} + \frac{8\tilde{C}^2 \V^2\log^2{T}}{m^2 T} + 14F\sqrt{\log{T}\E[R_T]}\; .
    \end{align*}
    Employing \Cref{lem:simple_cases_lemma} with $a=\E[R_T]$, $b=46\tilde{C}\V(F + \tilde{C}\V)\abs{\badrounds}\log{T} + 4\sqrt{56}\tilde{C}F\V\sqrt{\tilde{\gamma}T\log{T}} + 16\tilde{C}^2 \V^2\tilde{\gamma} + \frac{8\tilde{C}^2 \V^2\log^2{T}}{m^2 T}$, $c=14F$, and $d=\log{T}$, and dividing by $T$, results in
    \begin{align*}
        \E\sbrac{\frac{1}{T}\sum_{t\in\sbrac{T}}{\norm{\nabla_t}^2}} = \frac{\E[R_T]}{T} &\leq 8\sqrt{56}\tilde{C}F\V\sqrt{\frac{\tilde{\gamma}\log{T}}{T}} + 92\tilde{C}\V(F + \tilde{C}\V)\frac{\abs{\badrounds}\log{T}}{T} + \frac{32\tilde{C}^2 \V^2\tilde{\gamma}}{T} \\ &\quad+ \frac{16\tilde{C}^2 \V^2\log^2{T}}{m^2 T^2} + 784F^2\frac{\log{T}}{T}\; ,
    \end{align*}
    which concludes the proof.
\end{proof}
