# Supplementary material for: Dynamic Byzantine-Robust Learning: Adapting to Switching Byzantine Workers
Source: arXiv:2402.02951 source file (2024-06-16)
Supplement: Supplementary file 2 [file general_robust_aggr.tex]

\section{Analysis of \Cref{alg:method-new} with $(\delta,\kappa)$-robust Aggregator}\label{app:general}
In this section, we analyze \Cref{alg:method-new} with \textbf{Option 1}, which utilizes a general $(\delta,\kappa)$-robust aggregator. We first establish first and second order properties of our MLMC gradient estimator in Lemmas \ref{lem:mlmc_1st_general} and \ref{lem:mlmc_2nd_general}, respectively; then, we provide the proofs for the convex (\Cref{thm:convex}) and non-convex (\Cref{thm:nonconvex}) cases in \Cref{subapp:convex-general} and \Cref{subapp:nonconvex-general}, respectively.

Recall that \Cref{alg:method-new} with \textbf{Option 1} performs the following update rule for every $t\in\sbrac{T}$:
\begin{align}
    & J_t\sim\text{Geom}(\nicefrac{1}{2}) \nonumber \\
    & \widehat{g}_t^{j}\gets \A(\widebar{g}_{t,1}^{j},\ldots,\widebar{g}_{t,m}^{j}), \quad \text{ where } \widebar{g}_{t,i}^{j} = \frac{1}{2^{j}}\sum_{k=1}^{2^{j}}{\nabla F(x_t; \xi_{t,i}^{k})} \text{ for every } i\in\G_t \text{ if } t\notin\badrounds \label{eq:robust_aggregated_grad} \\
    & g_t \gets  \widehat{g}_t^{0} + \begin{cases}
        2^J_t\brac{\widehat{g}_t^{J_t} - \widehat{g}_t^{J_t-1}}, &\text{if } J_t\leq\Jmax\coloneqq\floor{\log{T}} \text{ and } \Ecal_t(J_t) \text{ holds} \\
        0, &\text{otherwise}
    \end{cases} \label{eq:mlmc_agg} \\
    & x_{t+1} \gets \proj{\K}{x_t - \eta_t g_t }\; , \nonumber
\end{align}
where the associated event $\Ecal_t(J_t)$ in this scenario is defined as,
\begin{equation}\label{eq:event_E_option1}
    \Ecal_t(J_t)\coloneqq \cbrac{\lVert \widehat{g}_t^{J_t} - \widehat{g}_t^{J_t-1}\rVert\leq 3C\V\sqrt{\frac{\gamma}{2^{J_t}}}}, \quad C=\sqrt{8\log\brac{4m^2 T}}, \enskip \gamma = \kappa + \frac{2\kappa+1}{m}\; .
\end{equation}

\begin{lemma}[MLMC Bias -- General Robust Aggregator]\label{lem:mlmc_1st_general}
    Consider the MLMC gradient estimator as defined in \Cref{eq:mlmc_agg}. For every $t\notin\badrounds$, it holds that
    \[
        \E_{t-1}[g_t] = \E_{t-1}[\widehat{g}_t^{\Jmax}] - y_t\; ,
    \]
    where $y_t$ satisfies: 
    % \begin{equation*}
        % \E\lVert{\widehat{g}_t^{\Jmax} - \nabla_t\rVert}^2 \leq \RD{...}\; ,
    % \end{equation*}
    % and $y_t$ is bounded as,
    \[
        \norm{y_t} \leq \frac{4\V\sqrt{2(4\kappa + 1)}\log{T}}{mT}\; .
    \]
\end{lemma}
\begin{proof}
    By explicitly writing the expectation w.r.t $J_t$, we have
    \begin{equation}\label{eq:mlmc_exp}
        \E_{t-1}[g_t] = \sum_{j=1}^{\infty}{2^{-j}\cdot \E_{t-1}\sbrac{\widehat{g}_t^{0} + 2^{j}\brac{\widehat{g}_t^{j} - \widehat{g}_t^{j-1}}\mathbbm{1}_{\cbrac{j\leq\Jmax}\cap\Ecal_t(j)}}} = \E_{t-1}[\widehat{g}_t^{0}] + \sum_{j=1}^{\Jmax}{\E_{t-1}\sbrac{\brac{\widehat{g}_t^{j} - \widehat{g}_t^{j-1}}\mathbbm{1}_{\Ecal_t(j)}}}\; .
    \end{equation}
    Utilizing \Cref{lem:expectation_indicator}, we can express each term in the sum as,
    \[
        \E_{t-1}\sbrac{\brac{\widehat{g}_t^{j} - \widehat{g}_t^{j-1}}\mathbbm{1}_{\Ecal_t(j)}} = \E_{t-1}\sbrac{\widehat{g}_t^{j} - \widehat{g}_t^{j-1}} - \E_{t-1}\sbrac{\widehat{g}_t^{j} - \widehat{g}_t^{j-1} | \Ecal_t(j)^c}\prob_{t-1}(\Ecal_t(j)^{c})\; .
    \]
    Denote the last term in the R.H.S by $z_t^{j}\coloneqq \E_{t-1}\sbrac{\widehat{g}_t^{j} - \widehat{g}_t^{j-1} | \Ecal_t(j)^c}\prob_{t-1}(\Ecal_t(j)^{c})$. Substituting this back into \Cref{eq:mlmc_exp}, we obtain:
    \begin{align}
        \E_{t-1}[g_t] &= \E_{t-1}[\widehat{g}_t^{0}] + \sum_{j=1}^{\Jmax}{\brac{\E_{t-1}[\widehat{g}_t^{j} - \widehat{g}_t^{j-1}] - z_t^{j}}} = \E_{t-1}[\widehat{g}_t^{\Jmax}] - y_t \nonumber \; ,
    \end{align}
    where $y_t = \sum_{j=1}^{\Jmax}{z_t^{j}}$. Our objective is to bound $y_t$; note that for every $j=1,\ldots,\Jmax$, we can bound $z_t^{j}$ using Jensen's inequality as follows:
    \begin{align*}
        \lVert{z_t^{j}\rVert} &= \norm{\E_{t-1}\sbrac{\widehat{g}_t^{j} - \widehat{g}_t^{j-1} | \Ecal_t(j)^c}\prob_{t-1}(\Ecal_t(j)^{c})} \leq \E_{t-1}\sbrac{\lVert \widehat{g}_t^{j} - \widehat{g}_t^{j-1} \rVert | \Ecal_t(j)^c}\prob_{t-1}(\Ecal_t(j)^c)\; .
    \end{align*}
    We will show that $\lVert{\widehat{g}_t^{j} - \widehat{g}_t^{j-1}\rVert}$ is bounded, and that the event $\Ecal_t(j)^{c}$ has a low probability.  

    By item 1 of \Cref{lem:core_lemma}, for every $j=0,\ldots,\Jmax$ it holds that $\lVert{\widehat{g}_t^{j} - \nabla_t\rVert}\leq \V\sqrt{2(4\kappa + 1)}$, which implies that $\lVert{ \widehat{g}_t^{j} - \widehat{g}_t^{j-1}\rVert}\leq \lVert{\widehat{g}_t^{j} - \nabla_t\rVert} + \lVert{\widehat{g}_t^{j-1} - \nabla_t\rVert}\leq 2\V\sqrt{2(4\kappa + 1)}$. In addition, by item 2 of \Cref{lem:core_lemma}, we have that
    \[
        \prob_{t-1}\brac{\lVert \widehat{g}_t^{j} - \nabla_t\rVert \leq C\V\sqrt{\frac{\gamma}{2^{j}}}} \geq 1-\frac{1}{mT}, \quad \forall j=0,\ldots,\Jmax\; . 
    \]
    This bound, in conjunction with the union bound, allows us to bound $\prob_{t-1}(\Ecal_t(j)^c)$ as,
    % Plugging this bound back gives:
    % \[
    %     \lVert{z_t^{j}\rVert} \leq 2\V\sqrt{2(4\kappa + 1)}\cdot\prob_{t-1}(\Ecal_t(j)^c)\; .
    % \]
    % Applying \RD{Lemma ...} in conjunction with the union bound enable to bound $\prob_{t-1}(\Ecal_t(j)^c)$ as,
    \begin{align*}
        \prob_{t-1}(\Ecal_t(j)^c) &= \prob_{t-1}\brac{\lVert \widehat{g}_t^{j} - \widehat{g}_t^{j-1}\rVert> 3C\V\sqrt{\frac{\gamma}{2^{j}}}}  \\ &\leq\prob_{t-1}\brac{\lVert \widehat{g}_t^{j} - \widehat{g}_t^{j-1}\rVert> (1 + \sqrt{2})C\V\sqrt{\frac{\gamma}{2^{j}}}} \\ &\leq\prob_{t-1}\brac{\cbrac{\lVert \widehat{g}_t^{j} - \nabla_t\rVert> C\V\sqrt{\frac{\gamma}{2^{j}}}}\bigcup \cbrac{\lVert \widehat{g}_t^{j-1} - \nabla_t \rVert> C\V\sqrt{\frac{\gamma}{2^{j-1}}}}} \\ &\leq \prob_{t-1}\brac{\lVert \widehat{g}_t^{j} - \nabla_t\rVert> C\V\sqrt{\frac{\gamma}{2^{j}}}} + \prob_{t-1}\brac{\lVert \widehat{g}_t^{j-1} - \nabla_t\rVert> C\V\sqrt{\frac{\gamma}{2^{j-1}}}} \\ &\leq \frac{1}{mT} + \frac{1}{mT} = \frac{2}{mT}\; .
    \end{align*}
    Combining the bounds on $\lVert{\widehat{g}_t^{j} - \widehat{g}_t^{j-1}\rVert}$ and $\prob_{t-1}(\Ecal_t(j)^c)$ gives:
    \[
        \lVert z_t^{j}\rVert \leq 2\V\sqrt{2(4\kappa + 1)}\cdot\frac{2}{mT} = \frac{4\V\sqrt{2(4\kappa + 1)}}{mT}\; ,
    \]
    which implies, by the triangle inequality, the following bound on $y_t$:
    \[
        \norm{y_t} \leq \sum_{j=1}^{\Jmax}{\lVert z_t^{j}\rVert} \leq \frac{4\V\sqrt{2(4\kappa + 1)}}{mT}\Jmax \leq \frac{4\V\sqrt{2(4\kappa + 1)}\log{T}}{mT}\; ,
    \]
    where we used $\Jmax\leq\log{T}$.
\end{proof}

Moving beyond the first-order analysis, we introduce a bound on the expected squared distance between the aggregated gradients and the true gradient. Subsequently, we provide a second-order bound for the MLMC gradient estimator.

\begin{lemma}\label{lem:2nd_order_aggr}
    Consider $\widehat{g}_t^{j}$ as defined in \Cref{eq:robust_aggregated_grad}. For every $j=0,\ldots,\Jmax\coloneqq\floor{\log{T}}$,
    \[
        \E\lVert{\widehat{g}_t^{j} - \nabla_t}\rVert^2 \leq \frac{5C^2 \V^2 \gamma}{2^j}\; .
    \]
\end{lemma}
\begin{proof}
    By item 2 of \Cref{lem:core_lemma}, it holds with probability at least $1-\nicefrac{1}{mT}$ that 
    \[
        \lVert{\widehat{g}_t^{j} - \nabla_t}\rVert^2 \leq \frac{C^2\V^2\gamma}{2^j}\; .
    \]
    In addition, item 1 of \Cref{lem:core_lemma} implies that $\lVert{\widehat{g}_t^{j} - \nabla_t\rVert}^2 \leq 2(4\kappa+1)\V^2$, deterministically. Combining these results, by the law of total expectation, it holds that 
    \begin{equation*}
        \E\lVert{\widehat{g}_t^{j} - \nabla_t}\rVert^2 \leq \frac{C^2 \V^2 \gamma}{2^j} + 2(4\kappa + 1)\V^2\cdot\frac{1}{mT} \leq \frac{C^2 \V^2 \gamma}{2^{j}} + \frac{4C^2 \V^2 \gamma}{2^j} = \frac{5C^2 \V^2 \gamma}{2^j}\; ,
    \end{equation*}
    where the last inequality follows from $\frac{2(4\kappa + 1)\V^2}{mT}\leq 4\brac{\kappa + \frac{2\kappa + 1}{m}}\frac{\V^2}{T}\leq \frac{4C^2\V^2 \gamma}{2^{j}}$ as $C^2\geq 1$ and $2^{j}\leq T$ for every $j=0,\ldots,\floor{\log{T}}$.
\end{proof}

\begin{lemma}[MLMC Variance -- General Robust Aggregator]\label{lem:mlmc_2nd_general}
    Consider the MLMC gradient estimator as defined in \Cref{eq:mlmc_agg}. For every $t\in\sbrac{T}$:
    \begin{equation*}
        \E\norm{g_t - \nabla_t}^2 \leq 28C^2\V^2\gamma\log{T}\; .
    \end{equation*}
\end{lemma}
\begin{proof}
    % Considering $\widehat{g}_t^{j}$ as defined in \Cref{eq:robust_aggregated_grad}, we start with bounding $\E\lVert \widehat{g}_t^{j} - \nabla_t\rVert^2$ for every $j=0,\ldots,\Jmax$. By item 2 of \Cref{lem:core_lemma}, it holds with probability at least $1-\nicefrac{1}{mT}$ that 
    % \[
    %     \lVert{\widehat{g}_t^{j} - \nabla_t}\rVert^2 \leq \frac{C^2\V^2\gamma}{2^j}\; .
    % \]
    % In addition, item 1 of \Cref{lem:core_lemma} implies that $\lVert{\widehat{g}_t^{j} - \nabla_t\rVert}^2 \leq 2(4\kappa+1)\V^2$, deterministically. Combining these results, by the law of total expectation, it holds that 
    % \begin{equation}\label{eq:aggr_grad_j}
    %     \E\lVert{\widehat{g}_t^{j} - \nabla_t}\rVert^2 \leq \frac{C^2 \V^2 \gamma}{2^j} + 2(4\kappa + 1)\V^2\cdot\frac{1}{mT} \leq \frac{C^2 \V^2 \gamma}{2^{j}} + \frac{4C^2 \V^2 \gamma}{2^j} = \frac{5C^2 \V^2 \gamma}{2^j}\; ,
    % \end{equation}
    % where the last inequality follows from $\frac{2(4\kappa + 1)\V^2}{mT}\leq 4\brac{\kappa + \frac{2\kappa + 1}{m}}\frac{\V^2}{T}\leq \frac{4C^2\V^2 \gamma}{2^{j}}$ as $C^2\geq 1$ and $2^{j}\leq T$ for every $j=0,\ldots,\floor{\log{T}}$.
    Explicitly writing the expectation w.r.t. $J_t$ gives:
    \begin{align}\label{eq:mlmc_second_moment_explicit}
        \E\norm{g_t - \nabla_t}^2 &= \sum_{j=1}^{\infty}{2^{-j}\E\norm{\widehat{g}_t^{0} + 2^{j}\brac{\widehat{g}_t^{j} - \widehat{g}_t^{j-1}}\mathbbm{1}_{\cbrac{j\leq\Jmax}\cap\Ecal_t(j)}}^2} \nonumber \\ &\leq 2\sum_{j=1}^{\infty}{2^{-j}\E\norm{\widehat{g}_t^{0} - \nabla_t}^2} + 2\sum_{j=1}^{\Jmax}{2^{j}\E\sbrac{\lVert{\widehat{g}_t^{j} - \widehat{g}_t^{j-1}}\rVert^2\mathbbm{1}_{\Ecal_t(j)}}} \nonumber \\ &= 2\E\norm{\widehat{g}_t^{0} - \nabla_t}^2 + 2\sum_{j=1}^{\Jmax}{2^{j}\underbrace{\E\sbrac{\lVert{\widehat{g}_t^{j} - \widehat{g}_t^{j-1}}\rVert^2\mathbbm{1}_{\Ecal_t(j)}}}_{=(\dag)}}\; ,
    \end{align}
    where the inequality follows from $\norm{a+b}^2\leq 2\norm{a}^2 + 2\norm{b}^2$, and the last equality holds as $\sum_{j=1}^{\infty}{2^{-j}}=1$. Focusing on $\brac{\dag}$, by the law of total expectation, we have that
    \begin{align*}
        \E\sbrac{\lVert{\widehat{g}_t^{j} - \widehat{g}_t^{j-1}}\rVert^2\mathbbm{1}_{\Ecal_t(j)}} = \E\sbrac{\lVert{\widehat{g}_t^{j} - \widehat{g}_t^{j-1}}\rVert^2 | \Ecal_t(j)}\underbrace{\prob(\Ecal_t(j))}_{\leq 1} \leq \frac{9C^2 \V^2 \gamma}{2^{j}}\; ,
    \end{align*}
    where the inequality follows from the bound of $\lVert \widehat{g}_t^{j} - \widehat{g}_t^{j-1}\rVert$ under the event $\Ecal_t(j)$ (see \Cref{eq:event_E_option1}). Furthermore, by \Cref{lem:2nd_order_aggr}, we can bound $\E\lVert \widehat{g}_t^{0}-\nabla_t \rVert^2\leq 5C^2 \V^2\gamma$. Substituting these bounds back to \Cref{eq:mlmc_second_moment_explicit} finally gives:
    \begin{align*}
        \E\norm{g_t - \nabla_t}^2 &\leq 10C^2\V^2\gamma + 2\sum_{j=1}^{\Jmax}{2^j\cdot\frac{9C^2\V^2\gamma}{2^{j}}} \leq 10C^2\V^2\gamma + 18C^2\V^2\gamma\Jmax \leq 28C^2\V^2\gamma\log{T}\; ,
    \end{align*}
    where the last inequality follows from $\Jmax\leq\log{T}$.
\end{proof}

\subsection{Proof of \Cref{thm:convex}}\label{subapp:convex-general}
In this section we prove \Cref{thm:convex}, restated here for convenience. 
\convex*

\begin{proof}
    We adopt a similar proof strategy to that presented in Theorem 3.8 of \cite{alistarh2018byzantine}. By the convexity of $f$, the gradient inequality implies that 
    \begin{equation}\label{eq:bias-var-decomp}
        \sum_{t\in\sbrac{T}}{\brac{f(x_t) - f(x^*)}} \leq \sum_{t\in\sbrac{T}}{\nabla_t^\top(x_t - x^*)} = \sum_{t\in\sbrac{T}}{g_t^{\top}(x_t - x^*)} + \sum_{t\in\sbrac{T}}{\brac{\nabla_t - g_t}^\top(x_t - x^*)}\; .
    \end{equation}
    % \begin{equation}\label{eq:bias-var-decomp}
    %     \E\sbrac{\sum_{t\in\sbrac{T}}{f(x_t) - f(x^*)}} \leq \E\sbrac{\sum_{t\in\sbrac{T}}{\nabla_t^\top(x_t - x^*)}} = \underbrace{\E\sbrac{\sum_{t\in\sbrac{T}}{g_t^{\top}(x_t - x^*)}}}_{=(A)} + \underbrace{\E\sbrac{\sum_{t\in\sbrac{T}}{\brac{\nabla_t - g_t}^\top(x_t - x^*)}}}_{=(B)}\; .
    % \end{equation}
    Focusing on the first term in the R.H.S, by applying \Cref{lem:classical_psgd} with $x=x^*$, we have
    \begin{align}\label{eq:bound_on_regret_convex}
        \sum_{t\in\sbrac{T}}{g_t^\top(x_t - x^*)} &\leq \frac{1}{2\eta}\sum_{t\in\sbrac{T}}{\brac{\norm{x_t - x^*}^2 - \norm{x_{t+1} - x^*}^2}} + \sum_{t\in\sbrac{T}}{\brac{g_t^\top(x_t - x_{t+1}) - \frac{1}{2\eta}\norm{x_t - x_{t+1}}^2}} \nonumber \\ &\leq \frac{D^2}{2\eta} + \sum_{t\in\sbrac{T}}{\brac{g_t^\top(x_t - x_{t+1}) - \frac{1}{2\eta}\norm{x_t - x_{t+1}}^2}}\; ,
    \end{align}
    where the last inequality follows from a telescoping sum and $\norm{x_1 - x^*}^2\leq D^2$. On the other hand, by the smoothness of $f$, we can bound the L.H.S as follows:
    \begin{equation}\label{eq:lower_bound_on_regret}
        \sum_{t\in\sbrac{T}}{\brac{f(x_t) - f(x^*)}} \geq \sum_{t\in\sbrac{T}}{\brac{f(x_{t+1}) - f(x^*) - \nabla_t^\top(x_{t+1} - x_{t}) - \frac{L}{2}\norm{x_t - x_{t+1}}^2}}\; .
    \end{equation}
    Plugging \Cref{eq:bound_on_regret_convex,eq:lower_bound_on_regret} back into \Cref{eq:bias-var-decomp} yields:
    \begin{align*}
        \sum_{t\in\sbrac{T}}{\brac{f(x_{t+1}) - f(x^*)}} &\leq \frac{D^2}{2\eta} + \sum_{t\in\sbrac{T}}{\brac{(g_t - \nabla_t)^\top(x_t - x_{t+1}) - \brac{\frac{1}{2\eta} - \frac{L}{2}}\norm{x_t - x_{t+1}}^2}} \\ &\quad+ \sum_{t\in\sbrac{T}}{\brac{\nabla_t - g_t}^\top(x_t - x^*)} \\ &\leq \frac{D^2}{2\eta} + \sum_{t\in\sbrac{T}}{\brac{(g_t - \nabla_t)^\top(x_t - x_{t+1}) - \frac{1}{4\eta}\norm{x_t - x_{t+1}}^2}} + \sum_{t\in\sbrac{T}}{\brac{\nabla_t - g_t}^\top(x_t - x^*)} \\ &\leq \frac{D^2}{2\eta} + \eta\sum_{t\in\sbrac{T}}{\norm{g_t - \nabla_t}^2} + \sum_{t\in\sbrac{T}}{\brac{\nabla_t - g_t}^\top(x_t - x^*)}\; ,
    \end{align*}
    where the second inequality follows from $\frac{1}{2\eta} - \frac{L}{2}\geq \frac{1}{4\eta}$ as $\eta\leq \frac{1}{2L}$ , and the final inequality uses Young's inequality, namely, $a^\top b - \frac{1}{2}\norm{b}^2\leq \frac{1}{2}\norm{a}^2$. By taking expectation, 
    \begin{equation}\label{eq:pre_final_convex}
        \E\sbrac{\sum_{t\in\sbrac{T}}{\brac{f(x_{t+1}) - f(x^*)}}} \leq \frac{D^2}{2\eta} + \eta\sum_{t\in\sbrac{T}}{\E\norm{g_t - \nabla_t}^2} + \underbrace{\E\sbrac{\sum_{t\in\sbrac{T}}{\brac{\nabla_t - g_t}^\top(x_t - x^*)}}}_{=(\star)}\; .
    \end{equation}

    \paragraph{Bounding $(\star)$. } We decompose the sum in $(\star)$ into two parts: one over bad rounds, $t\in\badrounds$, and the other over good rounds $t\in\sbrac{T}\setminus\badrounds$ (or simply $t\notin\badrounds$). Starting with the first part, we obtain using \Cref{lem:sum_of_inner_prods_cs},
    \begin{align}\label{eq:cs_badrounds}
        \E\sbrac{\sum_{t\in\badrounds}{(\nabla_t - g_t)^\top(x_t - x^*)}} &\leq \E\sbrac{\sqrt{\sum_{t\in\badrounds}{\norm{g_t - \nabla_t}^2}}\sqrt{\sum_{t\in\badrounds}{\norm{x_t - x^*}^2}}} \leq D\sqrt{\abs{\badrounds}}\sqrt{\sum_{t\in\badrounds}{\E\norm{g_t - \nabla_t}^2}}\; ,
    \end{align}
    where the second inequality follows from Jensen's inequality and $\norm{x_t - x^*}\leq D$. As for the second part, considering every $t\notin\badrounds$, since $x_t$ is measurable w.r.t $\F_t$, the application of the law of total expectation in conjunction with \Cref{lem:mlmc_1st_general} implies that
    \begin{align*}
        \E\sbrac{\brac{\nabla_t - g_t}^\top(x_t - x^*)} &= \E\sbrac{\E_{t-1}\sbrac{\brac{\nabla_t - g_t}^\top(x_t - x^*)}} \\ &= \E\sbrac{\brac{\nabla_t - \E_{t-1}[g_t]}^\top(x_t-x^*)} \\ &= \E\sbrac{\brac{\nabla_t - \widehat{g}_t^{\Jmax} + y_t}^\top(x_t - x^*)} ,
    \end{align*}
    where $\widehat{g}_t^{\Jmax}$ and $y_t$ satisfy, according to \Cref{lem:mlmc_1st_general,lem:2nd_order_aggr} (and $2^{\Jmax}\geq \nicefrac{T}{2}$),
    \begin{equation}\label{eq:dist_agg_Jmax_and_yt}
        \E\lVert{\widehat{g}_t^{\Jmax} - \nabla_t\rVert}^2 \leq \frac{5C^2\V^2\gamma}{2^{\Jmax}} \leq \frac{10C^2\V^2\gamma}{T}, \quad\text{ and }\quad \norm{y_t}^2 \leq \frac{32(4\kappa + 1)\V^2\log^2{T}}{m^2 T^2}\; .
    \end{equation}
    % and $y_t$ is bounded as,
    % \begin{equation}\label{eq:bound_on_yt}
        % \norm{y_t} \leq \frac{4\V\sqrt{2(4\kappa + 1)}\log{T}}{mT}\; .
    % \end{equation}
    Using \Cref{lem:sum_of_inner_prods_cs}, we have that 
    \begin{align}\label{eq:bias_cs}
        \E\sbrac{\sum_{t\notin\badrounds}{\brac{\nabla_t - g_t}^\top(x_t - x^*)}} &= \E\sbrac{\sum_{t\notin\badrounds}{\brac{\nabla_t - \widehat{g}_t^{\Jmax} + y_t}^\top(x_t - x^*)}} \nonumber \\ &\leq \E\sbrac{\sqrt{\sum_{t\notin\badrounds}{\lVert{\widehat{g}_t^{\Jmax} - \nabla_t}\rVert^2}}\sqrt{\sum_{t\notin\badrounds}{\norm{x_t - x^*}^2}}} + \E\sbrac{\sqrt{\sum_{t\notin\badrounds}{\norm{y_t}^2}}\sqrt{\sum_{t\notin\badrounds}{\norm{x_t - x^*}^2}}} \nonumber \\ &\leq D\sqrt{T}\sqrt{\sum_{t\notin\badrounds}{\E\lVert \widehat{g}_t^{\Jmax} - \nabla_t\rVert^2}} + D\sqrt{T}\sqrt{\sum_{t\notin\badrounds}{\E\norm{y_t}^2}}\; ,
    \end{align}
    where the last inequality follows from $\norm{x_t - x^*}\leq D$ and $\sqrt{T-\abs{\badrounds}}\leq\sqrt{T}$. Combining \Cref{eq:cs_badrounds,eq:bias_cs} enables to bound $(\star)$ as 
    \begin{align}\label{eq:bound_on_B_convex}
        \E\sbrac{\sum_{t\in\sbrac{T}}{\brac{\nabla_t - g_t}^\top(x_t - x^*)}} &= \E\sbrac{\sum_{t\in\badrounds}{\brac{\nabla_t - g_t}^\top(x_t - x^*)}} + \E\sbrac{\sum_{t\notin\badrounds}{\brac{\nabla_t - g_t}^\top(x_t - x^*)}} \nonumber \\ &\hspace{-1.2cm}\leq D\sqrt{\abs{\badrounds}}\sqrt{\sum_{t\in\badrounds}{\E\norm{g_t - \nabla_t}^2}} + D\sqrt{T}\sqrt{\sum_{t\notin\badrounds}{\E\lVert \widehat{g}_t^{\Jmax} - \nabla_t\rVert^2}} + D\sqrt{T}\sqrt{\sum_{t\notin\badrounds}{\E\norm{y_t}^2}}\; .
    \end{align}
    Plugging \Cref{eq:bound_on_B_convex} back into \Cref{eq:pre_final_convex} gives:
    \begin{align}
        \E\sbrac{\sum_{t\in\sbrac{T}}{\brac{f(x_{t+1}) - f(x^*)}}} &\leq \frac{D^2}{2\eta} + \eta\sum_{t\in\sbrac{T}}{\E\norm{g_t - \nabla_t}^2} + D\sqrt{\abs{\badrounds}}\sqrt{\sum_{t\in\badrounds}{\E\norm{g_t - \nabla_t}^2}} \nonumber \\ &\quad+ D\sqrt{T}\sqrt{\sum_{t\notin\badrounds}{\E\lVert \widehat{g}_t^{\Jmax} - \nabla_t\rVert^2}} + D\sqrt{T}\sqrt{\sum_{t\notin\badrounds}{\E\norm{y_t}^2}}\; . \nonumber 
    \end{align}
    % Utilizing \Cref{lem:self_boundness}, we have $\norm{\nabla_t}\leq 2L(f(x_t) - f^*)$, which implies that $\E\sbrac{\sum_{t\in\sbrac{T}}{\norm{\nabla_t}^2}} \leq 2L \E[R_T]$. Since $\eta\leq 1/4L$, we can bound $\eta \E\sbrac{\sum_{t\in\sbrac{T}}{\norm{\nabla_t}^2}}$ by $2\eta L\E[R_T]\leq \E[R_T]/2$. Plugging this bound, rearranging terms, and multiplying by $2$, we obtain
    % \begin{align}
    %      \E\sbrac{R_T} &\leq\frac{D^2}{\eta} + 2\eta\sum_{t\in\sbrac{T}}{\E\norm{g_t - \nabla_t}^2} + 2D\sqrt{\abs{\badrounds}}\sqrt{\sum_{t\in\badrounds}{\E\norm{g_t - \nabla_t}^2}} \nonumber \\ &\quad+ 2D\sqrt{T}\sqrt{\sum_{t\notin\badrounds}{\E\lVert \widehat{g}_t^{\Jmax} - \nabla_t\rVert^2}} + 2D\sqrt{T}\sqrt{\sum_{t\notin\badrounds}{\E\norm{y_t}^2}}\; .\nonumber
    % \end{align}
    Bounding $\E\lVert g_t - \nabla_t\rVert^2$, $\E\lVert \widehat{g}_t^{\Jmax} - \nabla_t\rVert^2$, and $\E\lVert y_t\rVert^2$ using \Cref{lem:mlmc_2nd_general} and \Cref{eq:dist_agg_Jmax_and_yt}, yields:
    \begin{align*}
        \E\!\sbrac{\sum_{t\in\sbrac{T}}{\brac{f(x_{t+1}) - f(x^*)}}} &\leq \frac{D^2}{2\eta} + \eta\sum_{t\in\sbrac{T}}{28 C^2\V^2\gamma\log{T}} + D\sqrt{\abs{\badrounds}}\sqrt{\sum_{t\in\badrounds}{28 C^2\V^2\gamma\log{T}}} \\ &\quad+ D\sqrt{T}\sqrt{\sum_{t\notin\badrounds}{\frac{10C^2\V^2\gamma}{T}}} + D\sqrt{T}\sqrt{\sum_{t\notin\badrounds}{\frac{32(4\kappa + 1)\V^2 \log^2{T}}{m^2 T^2}}} \\ &\leq \frac{1}{2}\!\brac{\frac{D^2}{\eta} + 64\eta C^2\V^2\gamma T\log{T}} + 6CD\V\sqrt{\gamma\log{T}}\abs{\badrounds} {+} 4CD\V\sqrt{\gamma T} {+} 8D\V\sqrt{\frac{\gamma}{m}}\log{T} \; ,
    \end{align*}
    where in the last inequality we used $\frac{4\kappa + 1}{m}\leq 2\gamma$ and $\abs{\sbrac{T}\setminus\badrounds}\leq T$. Since $\eta = \min\cbrac{\frac{D}{8C\V\sqrt{\gamma T\log{T}}}, \frac{1}{2L}}$, applying \Cref{lem:lr_min_of_2_lrs} with $a= D^2, b=64C^2\V^2\gamma T\log{T}$, and $c=2L$, allows us to bound the sum of the first two terms as follows
    \[
        \frac{D^2}{\eta} + 64\eta C^2\V^2\gamma T\log{T} \leq 16CD\V\sqrt{\gamma T\log{T}} + 2LD^2\; .
    \]
    Substituting this bound back yields:
    \begin{align*}
        \E\sbrac{\sum_{t\in\sbrac{T}}{\brac{f(x_{t+1}) - f(x^*)}}} &\leq 8CD\V\sqrt{\gamma T\log{T}} + LD^2 + 6CD\V\sqrt{\gamma\log{T}}\abs{\badrounds} + 4CD\V\sqrt{\gamma T} + 8D\V\sqrt{\frac{\gamma}{m}}\log{T}\; .
    \end{align*}
    Finally, dividing both sides by $T$ and utilizing Jensen's inequality concludes the proof,
    \begin{align*}
        \E\sbrac{f(\widebar{x}_T) - f(x^*)} &\leq \frac{1}{T}\E\sbrac{\sum_{t\in\sbrac{T}}{\brac{f(x_{t+1}) - f(x^*)}}} \\ &\leq 8CD\V\sqrt{\frac{\gamma\log{T}}{T}} + 6CD\V\sqrt{\gamma\log{T}}\frac{\abs{\badrounds}}{T} + 4CD\V\sqrt{\frac{\gamma}{T}} + 8D\V\sqrt{\frac{\gamma}{m}}\frac{\log{T}}{T} + \frac{LD^2}{T}\; .
    \end{align*}
\end{proof}

\subsection{Proof of \Cref{thm:nonconvex}}\label{subapp:nonconvex-general}
Having established the proof for the convex case, we now move on to proving convergence in the non-convex scenario, proving \Cref{thm:nonconvex}, presented here for ease of reference. Recall that in the non-convex case, we consider unconstrained minimization, and thus the update rule becomes $x_{t+1} = x_{t} - \eta g_t$.
\nonconvex*

\begin{proof}
    Let the sum of squared gradient norms be denoted as $R_T = \sum_{t\in\sbrac{T}}{\norm{\nabla_t}^2}$. By the $L$-smoothness of $f$, it holds that 
    \begin{align*}
        f(x_{t+1}) &\leq f(x_t) - \eta g_t^\top\nabla_t + \frac{L\eta^2}{2}\norm{g_t}^2 = f(x_t) - \eta\norm{\nabla_t}^2 - \eta\brac{g_t - \nabla_t}^\top\nabla_t + \frac{L\eta^2}{2}\norm{g_t}^2\; .
    \end{align*}
    Adding $\eta\norm{\nabla_t}^2$ to both sides and then dividing by $\eta$ yields:
    \begin{align*}
        \norm{\nabla_t}^2 \leq \frac{f(x_t) - f(x_{t+1})}{\eta} + \brac{\nabla_t - g_t}^\top\nabla_t + \frac{L\eta}{2}\norm{g_t}^2
    \end{align*}
    Summing over $t\in\sbrac{T}$, employing the inequality $\norm{g_t}^2\leq 2\norm{g_t - \nabla_t}^2 + 2\norm{\nabla_t}^2$, and taking expectation results in:
    \begin{align}\label{eq:regret_bound_nonconvex}
        \E[R_T] &\leq \frac{1}{\eta}\sum_{t\in\sbrac{T}}{\E\sbrac{f(x_t) - f(x_{t+1})}} + \sum_{t\in\sbrac{T}}{\E\sbrac{\brac{\nabla_t - g_t}^\top\nabla_t}} + L\eta\sum_{t\in\sbrac{T}}{\E\norm{g_t - \nabla_t}^2} + L\eta \E[R_T] \nonumber \\ &\leq \frac{\Delta_1}{\eta} + \underbrace{\sum_{t\in\sbrac{T}}{\E\sbrac{\brac{\nabla_t - g_t}^\top\nabla_t}}}_{=(\star)} + L\eta\sum_{t\in\sbrac{T}}{\E\norm{g_t - \nabla_t}^2} + \frac{1}{4}\E[R_T]\; ,
    \end{align}
    where the final inequality results from the telescoping sum and $f(x_{1}) - f(x_{T+1})\leq \Delta_1$, with the condition that $\eta\leq\nicefrac{1}{4L}$
    \paragraph{Bounding $(\star)$. } We handle this term similarly to how we treated $(\star)$ in the proof of \Cref{thm:convex}. Specifically, we decompose the sum represented by $(\star)$ into two parts: one over bad rounds, where $t\in\badrounds$, and the other over good rounds, where $t\notin\badrounds$. Starting with the second part, since $\nabla_t$ is measurable w.r.t $\F_t$, the application of the law of total expectation in conjunction with \Cref{lem:mlmc_1st_general} implies that 
    \begin{align*}
        \E\sbrac{\brac{\nabla_t - g_t}^\top\nabla_t} &= \E\sbrac{\E_{t-1}\sbrac{\brac{\nabla_t - g_t}^\top\nabla_t}} = \E\sbrac{\brac{\nabla_t - \E_{t-1}[g_t]}^\top\nabla_t} = \E\sbrac{\brac{\nabla_t - \widehat{g}_t^{\Jmax} + y_t}^\top\nabla_t}\; ,
    \end{align*}
    where $\widehat{g}_t^{\Jmax}$ and $y_t$ satisfy \Cref{eq:dist_agg_Jmax_and_yt}. Thus, we have that
    \begin{align}\label{eq:bound_on_star}
        \sum_{t\in\sbrac{T}}{\E\sbrac{\brac{\nabla_t - g_t}^\top\nabla_t}} &= \sum_{t\in\badrounds}{\E\sbrac{\brac{\nabla_t - g_t}^\top\nabla_t}} + \sum_{t\notin\badrounds}{\E\sbrac{\brac{\nabla_t - g_t}^\top\nabla_t}} \nonumber \\ &= \sum_{t\in\badrounds}{\E\sbrac{(\nabla_t - g_t)^\top\nabla_t}} + \sum_{t\notin\badrounds}{\E\sbrac{(\nabla_t - \widehat{g}_t^{\Jmax} + y_t)^\top\nabla_t}} \nonumber \\ &\leq  \frac{1}{2}\sum_{t\in\badrounds}{\brac{\E\norm{g_t - \nabla_t}^2 + \E\norm{\nabla_t}^2}} + \frac{1}{2}\sum_{t\notin\badrounds}{\brac{\E\lVert{\widehat{g}_t^{\Jmax} - \nabla_t + y_t}\rVert^2 + \E\norm{\nabla_t}^2}} \nonumber \\ &\leq \frac{1}{2}\sum_{t\in\badrounds}{\E\norm{g_t - \nabla_t}^2} + \sum_{t\notin\badrounds}{\brac{\E\lVert\widehat{g}_t^{\Jmax} - \nabla_t\rVert^2 + \E\lVert{y_t}\rVert^2}} + \frac{1}{2}\E[R_T]\; ,
    \end{align}
    where the first inequality follows from Young's inequality, namely, $a^\top b\leq \frac{\norm{a}^2}{2} + \frac{\norm{b}^2}{2}$. Plugging \Cref{eq:bound_on_star} back into \Cref{eq:regret_bound_nonconvex} gives:
    \begin{align*}
        \E[R_T] &\leq \frac{\Delta_1}{\eta} + L\eta\sum_{t\in\sbrac{T}}{\E\norm{g_t - \nabla_t}^2} + \frac{1}{2}\sum_{t\in\badrounds}{\E\norm{g_t - \nabla_t}^2} + \sum_{t\notin\badrounds}{\brac{\E\lVert\widehat{g}_t^{\Jmax} - \nabla_t\rVert^2 + \E\lVert{y_t}\rVert^2}}  + \frac{3}{4}\E[R_T]\; .
    \end{align*}
    Subtracting $\frac{3}{4}\E[R_T]$ and then multiplying by $4$, we get 
    \begin{align*}
        \E[R_T] &\leq \frac{4\Delta_1}{\eta} + 4L\eta\sum_{t\in\sbrac{T}}{\E\norm{g_t - \nabla_t}^2} + 2\sum_{t\in\badrounds}{\E\norm{g_t - \nabla_t}^2} + 4\sum_{t\notin\badrounds}{\brac{\E\lVert\widehat{g}_t^{\Jmax} - \nabla_t\rVert^2 + \E\lVert{y_t}\rVert^2}}\; .
    \end{align*}
    Analogously to the proof of \Cref{thm:convex}, we bound $\E\lVert g_t - \nabla_t\rVert^2$, $\E\lVert \widehat{g}_t^{\Jmax} - \nabla_t\rVert^2$, and $\E\lVert y_t\rVert^2$ using \Cref{lem:mlmc_2nd_general} and \Cref{eq:dist_agg_Jmax_and_yt}, to obtain:
    \begin{align*}
        \E[R_T] &\leq \frac{4\Delta_1}{\eta} + 4L\eta\sum_{t\in\sbrac{T}}{28C^2 \V^2 \gamma\log{T}} + 2\sum_{t\in\badrounds}{28C^2 \V^2\gamma\log{T}} + 4\sum_{t\notin\badrounds}{\brac{\frac{10C^2 \V^2 \gamma}{T} + \frac{32(4\kappa + 1)\V^2\log^2{T}}{m^2 T^2}}} \\ &\leq 4\brac{\frac{\Delta_1}{\eta} + 36\eta L C^2\V^2\gamma T\log{T}} + 56C^2\V^2 \gamma\abs{\badrounds}\log{T} + 40C^2 \V^2 \gamma + \frac{256\V^2\gamma\log^2{T}}{mT} \; ,
    \end{align*}
    where in the second inequality we used $\frac{4\kappa+1}{m}\leq 2\gamma$ and $\abs{\sbrac{T}\setminus\badrounds}\leq T$. Since $\eta = \min\cbrac{\frac{\sqrt{\Delta_1/ L}}{6C\V\sqrt{\gamma T\log{T}}}, \frac{1}{4L}}$, applying \Cref{lem:lr_min_of_2_lrs} with $a= \Delta_1, b=36LC^2\V^2\gamma T\log{T}$, and $c=4L$, enables to bound the sum of the first two terms as
    \[
        \frac{\Delta_1}{\eta} + 36\eta L C^2\V^2\gamma T\log{T} \leq 12C\V\sqrt{L\Delta_1\gamma T\log{T}} + 4L\Delta_1\; .
    \]
    Plugging in this bound, we get:
    \begin{align*}
        \E[R_T] &\leq 48C\V\sqrt{L\Delta_1\gamma T\log{T}} + 16L\Delta_1 + 56C^2\V^2\gamma\abs{\badrounds}\log{T} + \frac{256\V^2\gamma\log^2{T}}{mT}\; .
    \end{align*}
    Finally, dividing by $T$ completes the proof as follows:
    \begin{align*}
        \frac{1}{T}\E\sbrac{\sum_{t\in\sbrac{T}}{\norm{\nabla_t}^2}} &\leq 48C\V\sqrt{\frac{L\Delta_1\gamma\log{T}}{T}} + 56C^2\V^2 \gamma\log{T}\frac{\abs{\badrounds}}{T} + \frac{16L\Delta_1}{T} + \frac{256\V^2\gamma\log^2{T}}{mT^2}\; .
    \end{align*}
\end{proof}

% After establishing the proof for the convex case, we proceed to prove \Cref{thm:nonconvex}, establishing convergence in the non-convex scenario. presented here for ease of reference
